# Supplementary material for: Safe Control Synthesis with Uncertain Dynamics and Constraints
Source: arXiv:2202.09557 source file (2022-09-30)
Supplement: Supplementary file 1 [file Appendix_1.tex]

\section{Probabilistic Safe Control with MVGP Assumption}
In this section, we assume the barrier functions follow the distribution as stated in Problem~\ref{prob: prob_clf_cbf} and system dynamics follows the matrix Variate Gaussian Process (MVGP) distribution as stated in \cite{dhiman2020control}. While the MVGP assumption is not useful for learning system dynamics using dropout neural network, it balances the efficiency and accuracy of learning the dynamics using GP based methods. From the MVGP assumption, $F(\boldsymbol{x})$ can be described by a three-parameter distribution $\mathcal{MN}(\tilde{F}, \bfA, \bfB)$, where $\tilde{F} \in \mathbb{R}^{(1+m) \times n}$ is the mean and $\bfA \in \mathbb{R}^{(m+1) \times (m+1)}, \bfB \in \mathbb{R}^{n \times n}$ are the covariance matrices of the rows and columns of $F^\top(\boldsymbol{x})$. 

\begin{lemma}[{\cite{Sun2017LearningSW}}]
\label{lemma: MVG_1}
Let $\bfX$ follow an MVG distribution
$\mathcal{MN}(\bfM, \bfA, \bfB)$. Then, $\textit{vec}(\bfX) \sim \mathcal{N} (\textit{vec}(\bfM), \bfB \otimes \bfA)$.
\end{lemma}

By Lemma~\ref{lemma: MVG_1}, we propose the following GP decomposition of the system dynamics,
\begin{equation}
    \textit{vec}(F(\boldsymbol{x})) \sim \mathcal{GP}(\textit{vec}(\tilde{F}(\boldsymbol{x})),\bfB(\boldsymbol{x},\boldsymbol{x}') \otimes \bfA)
\end{equation} 
where $\otimes$ denotes the Kronecker product.

In this section, we aim at synthesizing a safe controller via the following optimization problem:

\begin{equation}
\label{eq:mvgp_CLF_CBF_QP}
\begin{aligned}
& \min_{\boldsymbol{u} \in \calU,\delta \in \bbR}\,\, \|L(\boldsymbol{x})^\top(\boldsymbol{u} - \tilde{\boldsymbol{u}}(\boldsymbol{x}))\|^2 + \lambda \delta^2\\
% \boldsymbol{u}^T H \boldsymbol{u} + p_d \delta^2 \\
\mathrm{s.t.} \, \,  &\mathbb{P}(\textit{CBC}(\boldsymbol{x}, \boldsymbol{u}) \geq \zeta) \geq p,
\end{aligned}
\end{equation}

% \subsection{Probabilistic Safety Constraints}
\begin{proposition}
\label{prop:mvgp_cbc_mean_variance}
Assume that the extended class $\mathcal{K}$ function $\alpha_h$ is linear ($\alpha_h(h(\boldsymbol{x})) = a \cdot h(\boldsymbol{x}), a \in \mathbb{R}$), assume the barrier function $h$ and system dynamics $F$ are independent. Given $h(\boldsymbol{x}) \sim \mathcal{GP}(\tilde{h}(\boldsymbol{x}),K_h(\boldsymbol{x},\boldsymbol{x}'))$) and ($\textit{vec}(F(\boldsymbol{x})) \sim \mathcal{GP}(\textit{vec}(\tilde{F}(\boldsymbol{x})),\bfB(\boldsymbol{x},\boldsymbol{x}') \otimes \bfA)$). We compute the mean and variance of $\textit{CBC}(\boldsymbol{x},\boldsymbol{u})$:
\begin{equation}
\label{eq: mvgp_cbc_mean_variance}
\begin{aligned}
&\mathbb{E}[\textit{CBC}(\boldsymbol{x},\boldsymbol{u})] = \bfM_1 (\boldsymbol{x}) \bfM_2 (\boldsymbol{x}) \\
& \textit{Var}[\textit{CBC}(\boldsymbol{x},\boldsymbol{u}] = \bfM_2 ^\top(\boldsymbol{x}) \bfK_1 (\boldsymbol{x},\boldsymbol{x}) \bfM_2(\boldsymbol{x}) + \\
&\bfM_1(\boldsymbol{x}) \bfK_2 (\boldsymbol{x},\boldsymbol{x}) \bfM_1^\top(\boldsymbol{x})
\end{aligned}
\end{equation}
where 
\begin{equation*}
    \bfM_1(\boldsymbol{x}) = [a \quad \underline{\boldsymbol{u}}^\top \tilde{F}^\top(\boldsymbol{x})] \in \mathbb{R}^{1 \times (n+1)}
\end{equation*}
\begin{equation}
\label{eq:mvgp_mean_m2}
    \bfM_2(\boldsymbol{x}) = \begin{bmatrix}
        \tilde{h}(\boldsymbol{x}) \\
        \nabla_{\boldsymbol{x}} \tilde{h}(\boldsymbol{x})
    \end{bmatrix} \in \mathbb{R}^{(n+1) \times 1}
\end{equation}

\begin{equation}
\label{eq:mvgp_covariance_k1}
    \bfK_1(\boldsymbol{x},\boldsymbol{x}') = \begin{bNiceArray}{c|ccc}[margin]
0 & 0 & \cdots & 0 \\
\hline
0 & \Block{3-3}{\bfB^\top(\boldsymbol{x},\boldsymbol{x}') \otimes \underline{\boldsymbol{u}}^\top \bfA^\top \underline{\boldsymbol{u}}}  & &  \\
\vdots& & \hspace*{2cm} & \\
0 & & & 
\end{bNiceArray} \in \mathbb{R}^{(n+1) \times (n+1)}
\end{equation}

\begin{equation}
\label{eq:mvgp_covariance_k2}
    \bfK_2(\boldsymbol{x},\boldsymbol{x}') =     \begin{bmatrix}
    \begin{aligned}
        K_h(\boldsymbol{x},\boldsymbol{x}')&, \nabla_{\boldsymbol{x}} K_h(\boldsymbol{x},\boldsymbol{x}')\\
        \nabla_{\boldsymbol{x}} K_h(\boldsymbol{x},\boldsymbol{x}')^\top&, \mathcal{H}_{\boldsymbol{x},\boldsymbol{x}}K_h(\boldsymbol{x},\boldsymbol{x}') 
    \end{aligned}
    \end{bmatrix} \in \mathbb{R}^{(n+1) \times (n+1)}
\end{equation}
and $\calH_{\boldsymbol{x},\boldsymbol{x}}$ denotes the Hessian matrix. 
\end{proposition}

\begin{proof}
Since $\alpha_h(h(\boldsymbol{x})) = a \cdot h(\boldsymbol{x}), a \in \mathbb{R}$, the original control barrier constraint can be written as: 
\begin{equation}
\begin{aligned}
\label{eq:mvgp_cbf}
    \textit{CBC}(\boldsymbol{x},\boldsymbol{u}) &= [\nabla_{\boldsymbol{x}} h(\boldsymbol{x})]^\top f(\boldsymbol{x}) + [\nabla_{\boldsymbol{x}} h(\boldsymbol{x})]^\top g(\boldsymbol{x})\boldsymbol{u} + a h(\boldsymbol{x})   \\
     &=     [a \quad f^\top(\boldsymbol{x})+(g(\boldsymbol{x})\boldsymbol{u})^\top] \cdot\begin{bmatrix}
    h(\boldsymbol{x}) \\
    \nabla_{\boldsymbol{x}} h(\boldsymbol{x})
    \end{bmatrix} \\
    &= [a \quad \underline{\boldsymbol{u}}^\top F^\top (\boldsymbol{x})] \cdot\begin{bmatrix}
    h(\boldsymbol{x}) \\
    \nabla_{\boldsymbol{x}} h(\boldsymbol{x})
    \end{bmatrix}   
\end{aligned}
\end{equation}

\begin{lemma}[{\cite{Sun2017LearningSW}}]
\label{lemma: MVG_2}
    Let $\bfX$ follow an MVG distribution $\mathcal{MN}(\bfM, \bfA, \bfB)$ and let $\bfC \in \mathbb{R}^{d \times n}$ and $\bfD \in \mathbb{R}^{m \times d}$. Then,
    
    \begin{equation*}
    \begin{aligned}
       &\bfC \bfX \sim \mathcal{MN}(\bfC \bfM, \bfC \bfA \bfC^\top, \bfB); \\
       &\bfX \bfD \sim \mathcal{MN}(\bfD\bfC, \bfA , \bfD^\top \bfB \bfD)
    \end{aligned}
    \end{equation*}
\end{lemma}

%As the transposition is distributive over the Kronecker product, 

By Lemma~\ref{lemma: MVG_2}, for any given control input $\boldsymbol{u}$, the MVGP of $\underline{\boldsymbol{u}}^\top F^\top(\boldsymbol{x})$ is: 
\begin{equation}
    \underline{\boldsymbol{u}}^\top F^\top(\boldsymbol{x}) \sim \mathcal{MN}(\underline{\boldsymbol{u}}^\top \tilde{F}^\top(\boldsymbol{x}), \underline{\boldsymbol{u}}^\top\bfA^\top \underline{\boldsymbol{u}}, \bfB^\top)
\end{equation}
since $\underline{\boldsymbol{u}}^\top F^\top(\boldsymbol{x}) \in \mathbb{R}^{1 \times n}$ is a row vector, we have
\begin{equation}
    \underline{\boldsymbol{u}}^\top F^\top(\boldsymbol{x}) \sim \mathcal{GP}(\underline{\boldsymbol{u}}^\top \tilde{F}^\top(\boldsymbol{x}),\bfB^\top(\boldsymbol{x},\boldsymbol{x}') \otimes \underline{\boldsymbol{u}}^\top \bfA^\top \underline{\boldsymbol{u}}) 
\end{equation}
Now, we know $[a \quad \underline{\boldsymbol{u}}^\top F^\top (\boldsymbol{x})]$ in \eqref{eq:mvgp_cbf} is GP with mean $\bfM_1(\boldsymbol{x}) = [a \quad \underline{\boldsymbol{u}}^\top \tilde{F}^\top(\boldsymbol{x})]$ and kernel function $\bfK_1(\boldsymbol{x},\boldsymbol{x}')$ defined in \eqref{eq:mvgp_covariance_k1}. 

In our previous work~\cite{dhiman2020control}, it is shown that the gradient of a GP is also GP. Specifically, the barrier function gradient $\nabla_{\boldsymbol{x}}   h(\boldsymbol{x})$ is GP given that $h(\boldsymbol{x}) \sim \mathcal{GP}(M_h(\boldsymbol{x}),K_h(\boldsymbol{x},\boldsymbol{x}'))$, and
\begin{equation}
\begin{aligned}
    \begin{bmatrix}
        h(\boldsymbol{x}) \\
         \nabla_{\boldsymbol{x}} h(\boldsymbol{x})
    \end{bmatrix}
    \sim
    \mathcal{GP}(\bfM_2(\boldsymbol{x}),\bfK_2(\boldsymbol{x},\boldsymbol{x}'))
\end{aligned}
\end{equation}
where $\bfM_2(\boldsymbol{x})$ and $\bfK_2(\boldsymbol{x},\boldsymbol{x}')$ are defined in \eqref{eq:mvgp_mean_m2} and \eqref{eq:mvgp_covariance_k2} respectively.

In~\eqref{eq:mvgp_cbf}, we need to compute $\textit{CBC}(\boldsymbol{x},\boldsymbol{u})$ as a product of two independent GPs. By Lemma~\ref{lemma: gp_product}, we show that the result is a real-valued scalar distribution with mean $\mathbb{E}[\textit{CBC}(\boldsymbol{x},\boldsymbol{u})]$ and variance $\textit{Var}(\textit{CBC}(\boldsymbol{x},\boldsymbol{u}))$,

\begin{equation}
\label{eq:mvgp_cbc_mean}
    \mathbb{E}[\textit{CBC}(\boldsymbol{x},\boldsymbol{u})] = \bfM_1 (\boldsymbol{x}) \bfM_2 (\boldsymbol{x})
\end{equation}

\begin{equation}
\begin{aligned}
\label{eq:mvgp_cbc_var}
    \textit{Var}[\textit{CBC}(\boldsymbol{x},\boldsymbol{u}] = &\bfM_2 ^\top(\boldsymbol{x}) \bfK_1 (\boldsymbol{x},\boldsymbol{x}) \bfM_2(\boldsymbol{x}) + \\
    &\bfM_1(\boldsymbol{x}) \bfK_2 (\boldsymbol{x},\boldsymbol{x}) \bfM_1^\top(\boldsymbol{x})
\end{aligned}
\end{equation}

\end{proof}
 
\begin{proposition}
\label{prop:mvgp_socp}
Assume the mean and variance of the control barrier constraint in Proposition~\ref{prop:cbc_mean_variance} as \eqref{eq: cbc_mean_variance}, we can write \eqref{eq:CLF_CBF_QP_Gaussian} as a second order cone program as follows: 
\begin{equation}
\label{eq:mvgp_socp_form}
\begin{aligned}
    & \min_{\boldsymbol{u} \in \calU, \delta\in \mathbb{R},l\in \mathbb{R} } \, \, l \\
    \mathrm{s.t.} \, \, 
    &\delta - \mathbb{E}[\textit{CLC}(\boldsymbol{x},\boldsymbol{u})] \geq c(p)\|\textit{Var}[\textit{CLC}(\boldsymbol{x},\boldsymbol{u})\|_2
    \\
    &\zeta - \mathbb{E}[\textit{CBC}(\boldsymbol{x},\boldsymbol{u})] \leq -c(p)\|\textit{Var}[\textit{CBC}(\boldsymbol{x},\boldsymbol{u})\|_2 
     \\
    &\Bigg\| \begin{bmatrix} 2L(\boldsymbol{x})^\top(\boldsymbol{u}-\tilde{\boldsymbol{u}}(\boldsymbol{x}))\\ 2\sqrt{\lambda} \delta \\ l-1 \end{bmatrix} \Bigg\| \leq l+1.
    % (L^T (\hat{\boldsymbol{u}}-\hat{\boldsymbol{u}}_{ref}), l, 1) \\
    % &\in \mathcal{Q}^n_{rot}\\
\end{aligned}
\end{equation}
where $c(p) = \sqrt{\frac{p}{1-p}}$.
\end{proposition}
% \KL{Correction: This is not the chi-square distribution, consider hansen-wright equation or use cantelli's inequality directly}
\begin{proof}
Same as Proposition~\ref{prop:gaussian_socp}.

\end{proof}

% \begin{remark*}[Arbitrary relative degree in system dynamics]
% If the relative degree in~\eqref{eq: dynamic} is greater than $1$, we need to compute the products of more than two Gaussians, where the result distributions cannot be determined by Lemma~\ref{lemma: gp_product}. Instead, one can use Monte Carlo approximations to estimate the means and variances of $\textit{CBC}(\boldsymbol{x},\boldsymbol{u})$.
% \end{remark*}
