# Supplementary material for: Safe Control Synthesis with Uncertain Dynamics and Constraints
Source: arXiv:2202.09557 source file (2022-09-30)
Supplement: Supplementary file 2 [file Appendix_3.tex]

\section{Norm Sum as SOC Constraints}\label{sum_of_norms_soc}

\begin{lemma}
\label{lemma:sum_of_norms}
The convex problem:
\begin{equation*}
\label{eq:soc_need_convert}
\begin{aligned}
& \min_{\bfz \in \bbR^n}\,\, \boldsymbol{v}^\top \bfz\\
% \boldsymbol{u}^T H \boldsymbol{u} + p_d \delta^2 \\
\mathrm{s.t.} \, \,  &\|\bfA\bfz - \boldsymbol{a}\| + \|\bfB\bfz - \boldsymbol{b}\| \leq \boldsymbol{c}^\top \bfz
\end{aligned}
\end{equation*}
is equivalent to the second-order cone program:
\begin{equation*}
\label{eq:converted_SOC_constraint}
\begin{aligned}
& \min_{\bfz \in \bbR^n, p\in \mathbb{R}, q\in \mathbb{R}}\,\, \boldsymbol{v}^\top \bfz\\
% \boldsymbol{u}^T H \boldsymbol{u} + p_d \delta^2 \\
\mathrm{s.t.} \, \,  &\|\bfA\bfz - \boldsymbol{a}\| \leq p \\
& \|\bfB\bfz - \boldsymbol{b}\| \leq q \\
&  p+q \leq \boldsymbol{c}^\top \bfz.
\end{aligned}
\end{equation*}
\end{lemma}
%
% \marginJC{I think the proof is self-evident -- we can show it to the reviewers if they complain. Having the statement is still useful, as it simplifies the proof of our proposition earlier.}
%
%\begin{proof}
%We first introduce two auxiliary variable $p, q \in \mathbb{R}$. 

%$(\Rightarrow)$: Assume that the original constraint in \eqref{eq:soc_need_convert} is satisfied. By choosing $p = \|\bfA\bfz - \boldsymbol{a}\|$ and $q = \|\bfB\bfz - \boldsymbol{b}\|$, the constraints in \eqref{eq:converted_SOC_constraint} are all satisfied. 

%$(\Leftarrow)$: Assume that the constraints in \eqref{eq:converted_SOC_constraint} are all satisfied. We can write
%
%\begin{equation*}
 %   \|\bfA\bfz - \boldsymbol{a}\| + \|\bfB\bfz - %\boldsymbol{b}\| \leq p + q \leq \boldsymbol{c}^\top \bfz,
%\end{equation*}
%
%which implies the constraint in \eqref{eq:soc_need_convert} is also %satisfied.
%\end{proof}
