# Supplementary material for: Safe Control Synthesis with Uncertain Dynamics and Constraints
Source: arXiv:2202.09557 source file (2022-09-30)
Supplement: Supplementary file 3 [file Appendix_2.tex]

\section{Convert QP to SOCP}
\label{qp_to_socp}
\begin{proposition}
\label{prop:qp_convert_socp}
For a general CLF-CBF-QP problem as follows, 
\begin{equation}
\label{eq:QP_need_convert}
\begin{aligned}
& \min_{\boldsymbol{u} \in \calU,\delta \in \bbR}\,\, \|L(\boldsymbol{x})^\top(\boldsymbol{u} - \tilde{\boldsymbol{u}}(\boldsymbol{x}))\|^2 + \lambda \delta^2,\\
% \boldsymbol{u}^T H \boldsymbol{u} + p_d \delta^2 \\
\mathrm{s.t.} \, \,  &\textit{CLC}(\boldsymbol{x},\boldsymbol{u}) \leq \delta,  \textit{CBC}(\boldsymbol{x},\boldsymbol{u}) \geq 0,
\end{aligned}
\end{equation}
one can formulate it as a convex second-order cone program (SOCP) by reformulating the objective function as a constraint, which results in,
\begin{equation}
\label{eq:converted_SOCP}
\begin{aligned}
    & \min_{\boldsymbol{u} \in \calU, \delta\in \mathbb{R},l\in \mathbb{R} } \, \, l \\
    \mathrm{s.t.} \, \, &\textit{CLC}(\boldsymbol{x},\boldsymbol{u}) \leq \delta,  \textit{CBC}(\boldsymbol{x},\boldsymbol{u}) \geq 0, \\
    &\left\| \begin{bmatrix} 2L(\boldsymbol{x})^\top(\boldsymbol{u}-\tilde{\boldsymbol{u}}(\boldsymbol{x}))\\ 2\sqrt{\lambda} \delta \\ l-1 \end{bmatrix} \right\| \leq l+1.
\end{aligned}
\end{equation}
\end{proposition}

\begin{proof}
We first introduce a new variable $l$ so that the problem in \eqref{eq:QP_need_convert} is equivalent to
\begin{equation}
\label{eq:SOCP_error_bound}
\begin{aligned}
    & \min_{\boldsymbol{u} \in \calU, \delta\in \mathbb{R},l\in \mathbb{R} } \, \, l \\
    \text{s.t.} \, \, 
    &\textit{CLC}(\boldsymbol{x},\boldsymbol{u}) \leq \delta,  \textit{CBC}(\boldsymbol{x},\boldsymbol{u}) \geq 0, \\
    &\|L(\boldsymbol{x})^\top(\boldsymbol{u}-\tilde{\boldsymbol{u}}(\boldsymbol{x}))\|^2 + \lambda \delta^2 \leq l.
\end{aligned}
\end{equation}

The last constraint in \eqref{eq:SOCP_error_bound} corresponds to a rotated second-order cone, $\mathcal{Q}^n_{rot} \coloneqq \{(\boldsymbol{x}_{r},y_{r},z_{r}) \in \mathbb{R}^{n+2}\, | \,\|\boldsymbol{x}_{r}\|^2 \leq y_{r}z_{r}, y_{r} \geq 0, z_{r} \geq 0 \}$, which can be converted into a standard SOC constraint~\cite{alizadeh2003second},
\[
\left\| \begin{bmatrix} 2 \boldsymbol{x}_{r} \\ y_r - z_r\end{bmatrix} \right\| \leq y_r+z_r.
\]

Let $y_r = l$, $z_r = 1$ and consider the constraint $\|L(\boldsymbol{x})^\top(\boldsymbol{u}-\tilde{\boldsymbol{u}}(\boldsymbol{x}))\|^2 + \lambda \delta^2 \leq l$. Multiplying both sides by $4$ and adding $(l-1)^2$, makes the constraint equivalent to 
\[
4\| L(\boldsymbol{x})^\top (\boldsymbol{u}-\tilde{\boldsymbol{u}}(\boldsymbol{x})) \|^2 + 4\lambda\delta^2 + (l-1)^2 \leq (l+1)^2.
\]
Taking a square root on both sides, we end up with $\sqrt{ \|2L(\boldsymbol{x})^\top (\boldsymbol{u}-\tilde{\boldsymbol{u}}(\boldsymbol{x}))\|^2 + (2\sqrt{\lambda}\delta)^2 + (l-1)^2} \leq l+1$, which is equivalent to the third constraint in \eqref{eq:converted_SOCP}.
\end{proof}
